# Supplementary material for: Evaluating two-loop non-planar master integrals for Higgs + jet production with full heavy-quark mass dependence
Source: arXiv:1907.13156 source file (2020-01-31)
Supplement: Supplementary file 1 [file plotsappendix4.tex]

In this appendix we show the plots of all the integrals of our basis along the line joining the kinematical point $\textrm{P}_{\textrm{below}} = (s=2, t=-1, p_4^2=13/25)$  to $\textrm{P}_{\textrm{above}}=(6,-1,13/25)$, which are obtained using the expansion method. The blue and orange lines are the real and imaginary parts and the dots are values obtained with FIESTA for comparison. Note that the only noticeable mismatch is for $B_{68}^{(4)}$ and $B_{69}^{(4)}$, but is well inside the uncertainty produced by FIESTA (not reported here).
 
\begin{table}[h!]
	\begin{tabular}{ p{4cm}  p{4cm}  p{4cm}  p{4cm}}
        
        \img{1} & \img{2} & \img{3} & \img{4} \\
        
        \img{5} & \img{6} & \img{7} & \img{8} \\
        
        \img{9} & \img{10} & \img{11} & \img{12} \\
        
        \img{13} & \img{14} & \img{15} & \img{16} \\
        
        \img{17} & \img{18} & \img{19} & \img{20} \\
        
        \img{21} & \img{22} & \img{23} & \img{24} \\
        
        \img{25} & \img{26} & \img{27} & \img{28} \\
        
        \img{29} & \img{30} & \img{31} & \img{32} \\
        
        \img{33} & \img{34} & \img{35} & \img{36} 
\end{tabular}
\end{table}

\begin{table}[t!]
	\begin{tabular}{ p{4cm}  p{4cm}  p{4cm}  p{4cm}}
	
    	\img{37} & \img{38} & \img{39} & \img{40} \\
        
        \img{41} & \img{42} & \img{43} & \img{44} \\
        
        \img{45} & \img{46} & \img{47} & \img{48} \\
        
        \img{49} & \img{50} & \img{51} & \img{52} \\
        
        \img{53} & \img{54} & \img{55} & \img{56} \\
        
        \img{57} & \img{58} & \img{59} & \img{60} \\
        
        \img{61} & \img{62} & \img{63} & \img{64} \\
        
        \img{65} & \img{66} & \img{67} & \img{68} \\
        
        \img{69} & \img{70} & \img{71} & \img{72} \\
        
\end{tabular}
\end{table}

\FloatBarrier
